# Supplementary material for: Learning the Optimal Stopping for Early Classification within Finite Horizons via Sequential Probability Ratio Test
Source: arXiv:2501.18059 source file (2025-01-29)
Supplement: Supplementary file 1 [file Supplementary_ICNN.tex]

\section{On the choice of CFL algorithm.}\label{app:ICNN}

\paragraph{Convergence guarantee on the two-block ADMM algorithm.}
We used the two-block ADMM algorithm in \texttt{FIRMBOUND} for its consistent convex function estimation and faster convergence rate, $ \mathcal{O}\left(\frac{n^3 d^{1.5}}{\epsilon} + \frac{n^2 d^{2.5}}{\epsilon} + \frac{n d^3}{\epsilon}\right) $, where $n, d, \epsilon$ are the number of data points, dimensionality of the data, and desired error~\citeApp{Siahkamari2022CFL}, which is considerably more efficient than the traditional ADMM's $ \mathcal{O}\left(\frac{n^5 d^2}{\epsilon}\right) $.

\paragraph{Input-Convex Neural Networks as an estimator of the conditional probability.} 
As an additional method to estimate the conditional expectation, we experimented with Input-Convex Neural Networks (ICNN~\citeApp{Amos2017ICNN}). ICNNs, which employ non-negative weights and non-decreasing activation functions such as softplus, ensure that the learned function remains convex with respect to its inputs. This characteristic is advantageous in optimization problems, where convexity can facilitate more efficient and robust solutions. However, we observed that ICNNs are overly sensitive to data noise and have difficulty fitting even a simple parabola (Figure \ref{fig:ICNN}), making them unsuitable for real-world applications.

\begin{figure*}[htbp]
    \centerline{\includegraphics[width=14cm,keepaspectratio]{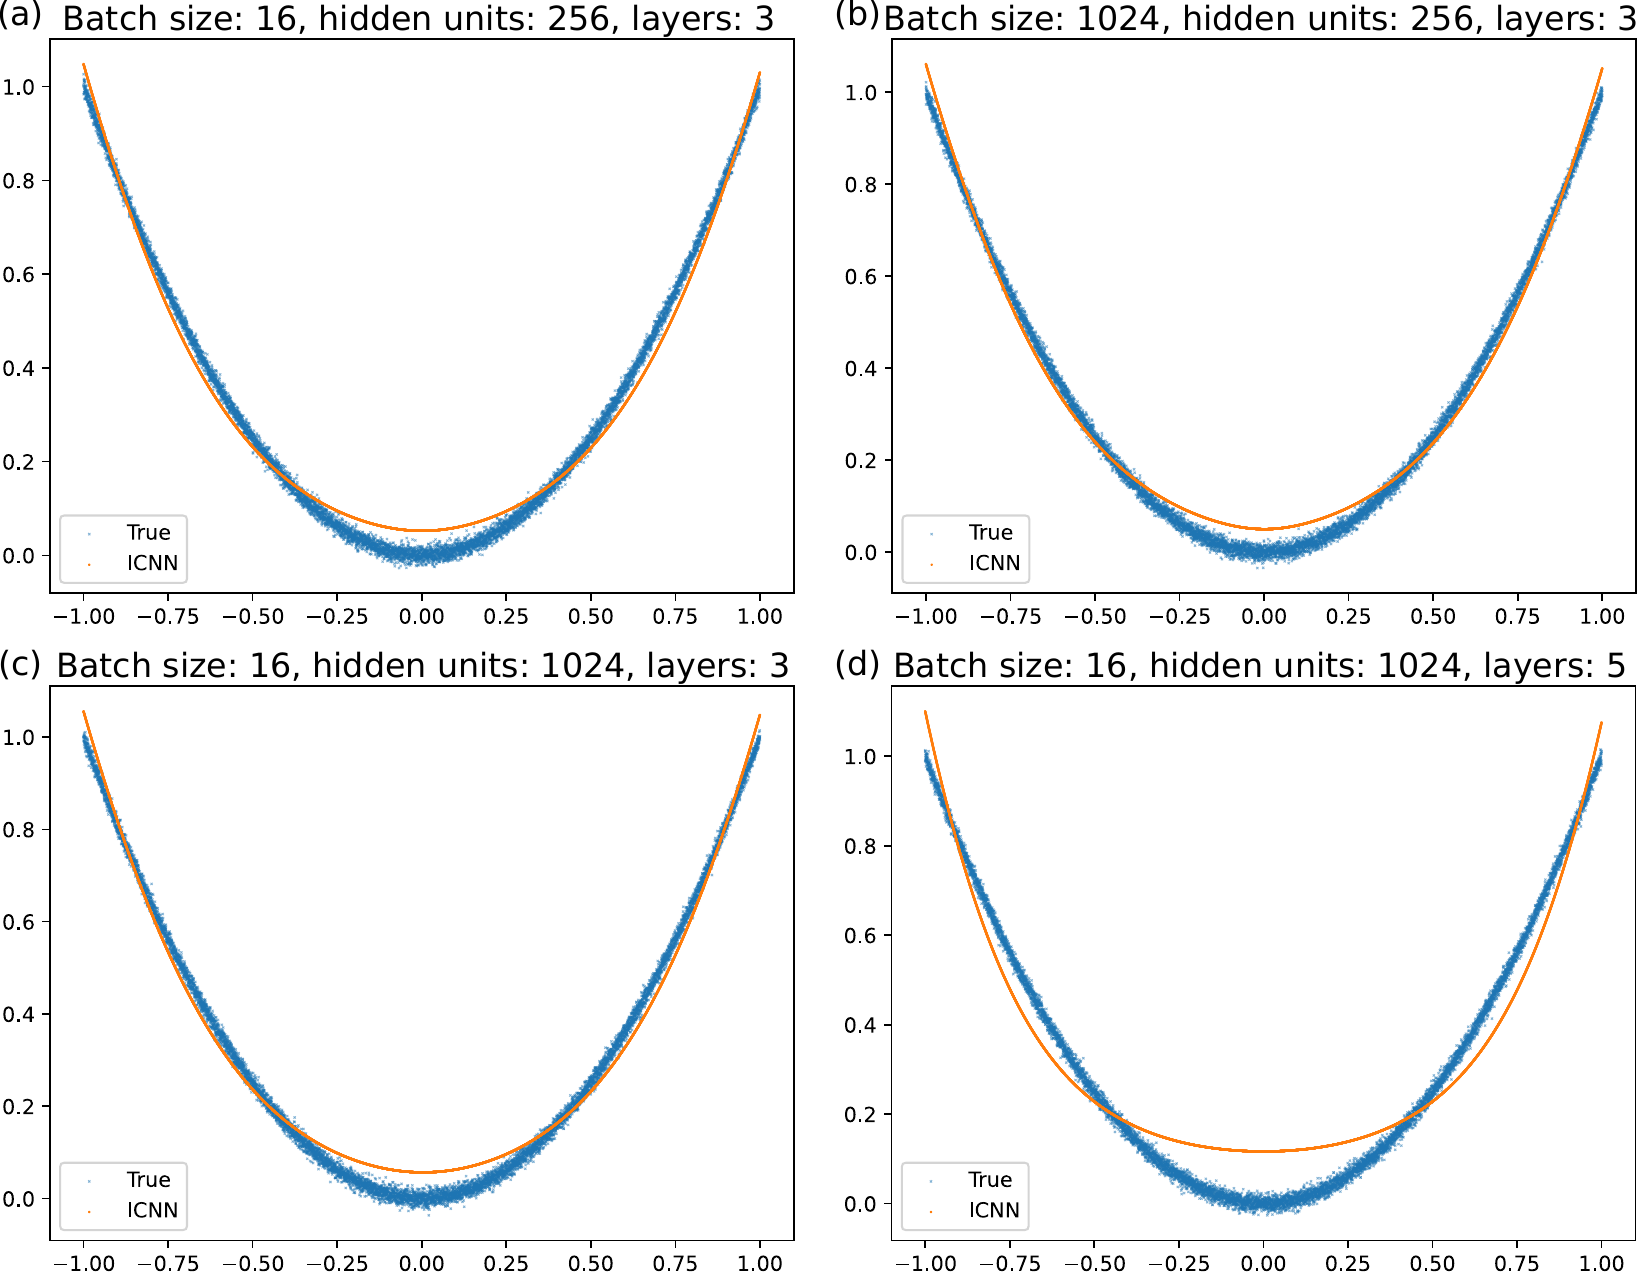}}
    \caption{ICNNs have difficulty fitting even a simple parabola.
        ICNNs are trained on a one-dimensional parabola. 
        The plot shows the perturbed one-dimensional parabola (blue) and its ICNN approximation (orange) after training for 50,000 iterations on 10,000 samples.
        The ground-truth parabola is defined as $y=x^2$ with $x + 0.01 \times \epsilon$, where $x \in [-1, 1]$, and $\epsilon$ is drawn from the standard Gaussian distribution)
        The learning rate decays by a factor of 0.5 every 20,000 iterations. 
        The ICNN has 3 or 5 linear layers with 256 or 1024 hidden units and a softplus activation for each and uses the Adam optimizer with the initial learning rate of 0.01, batch size of 16 or 1024, and no weight decay. The loss function is the mean squared error (MSE) loss.}
        \label{fig:ICNN}
\end{figure*}

\clearpage
