# Supplementary material for: Learning the Optimal Stopping for Early Classification within Finite Horizons via Sequential Probability Ratio Test
Source: arXiv:2501.18059 source file (2025-01-29)
Supplement: Supplementary file 2 [file Supplementary_domain_gap.tex]

\section{Domain Gap in UCF101 Prevents \texttt{FIRMBOUND} from Reaching the Global Minima}\label{app:domain_gap}
We would like to address the critical concern regarding FIRMBOUND's failure to achieve the global minima of the average a posteriori risk (AAPR) under the UCF101 dataset.

We have identified that the primary reason behind the failure to achieve the global minima on the UCF101 test dataset is the \textbf{domain gap} between the training and test datasets. 

\begin{figure*}[htbp]
\centerline{\includegraphics[width=7cm,keepaspectratio]{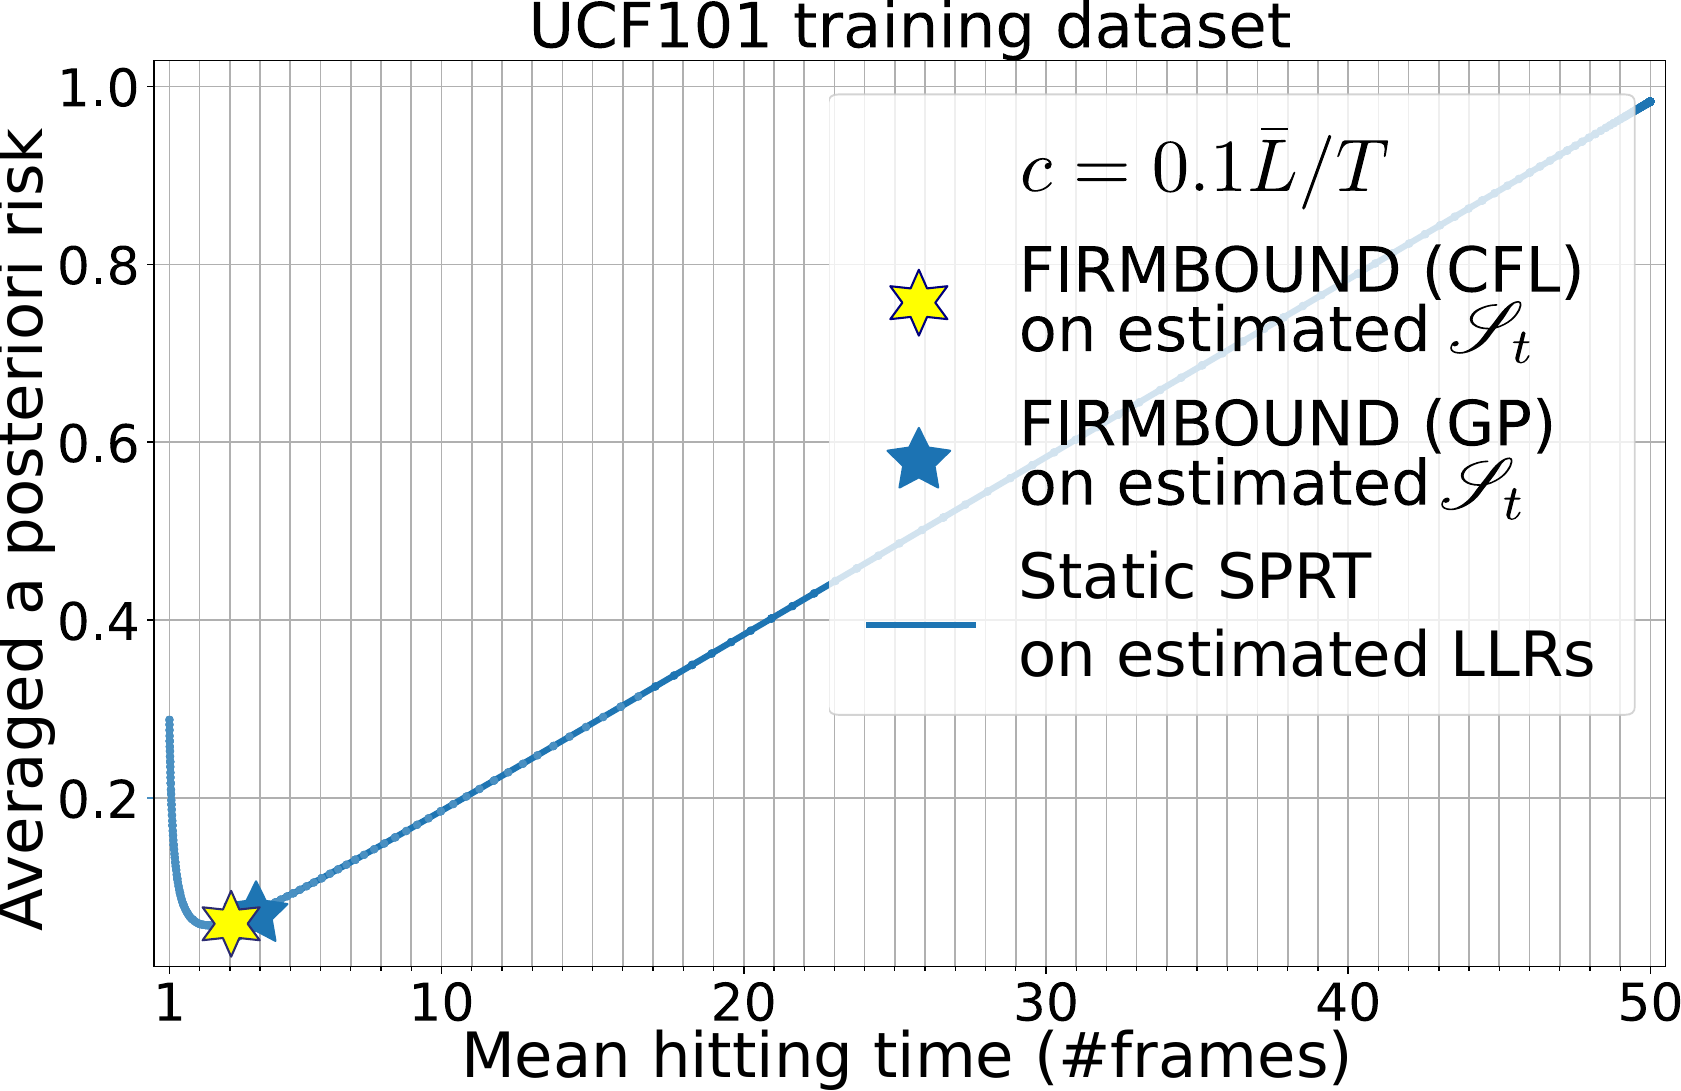}}
\caption{\textbf{Results on the training dataset of UCF101.} }
\end{figure*}
In our additional experiments, we observed that FIRMBOUND does achieve the global minima of AAPR on the UCF101 training dataset. This indicates that our method is capable of optimal performance when the training and test data distributions are aligned. However, the discrepancy between the training and test datasets in UCF101, which reflects a domain gap, has affected the generalizability of our results. 

Fig.~\ref{fig:UCF_domain_gap} illustrates the estimated LLR trajectories for two example classes from the UCF101 dataset. The red and blue trajectories represent the likelihood ratios for two different classes. The LLR trajectories for the training data (left panel) exhibit good separability between the two classes, with clear and distinct increases and decreases in LLR values. In contrast, the LLR trajectories for the test data (right panel) show significantly smaller angles and reduced class separation. The LLRs for the test data have smaller magnitudes and exhibit a delayed increase compared to the training data. This discrepancy indicates a domain gap between the training and test datasets. The smaller magnitude and delayed increase of LLRs in the test data lead to decision delays when applying decision boundaries learned from the training dataset. This phenomenon contributes to the observed failure in achieving the global minima of the average a posteriori risk (AAPR) on the UCF101 test dataset. 

In comparison, the SiW dataset exhibited minimal domain gap between its training and test datasets, as evidenced by consistent LLR trajectories (Fig.~\ref{fig:SiW_domain_gap}). This supports the interpretation that the delayed decision-making observed in the UCF101 dataset, and the successful minimization of AAPR on the SiW dataset, is attributable to the domain gap present in UCF101.

\begin{figure*}[htbp]
\centerline{\includegraphics[width=14cm,keepaspectratio]{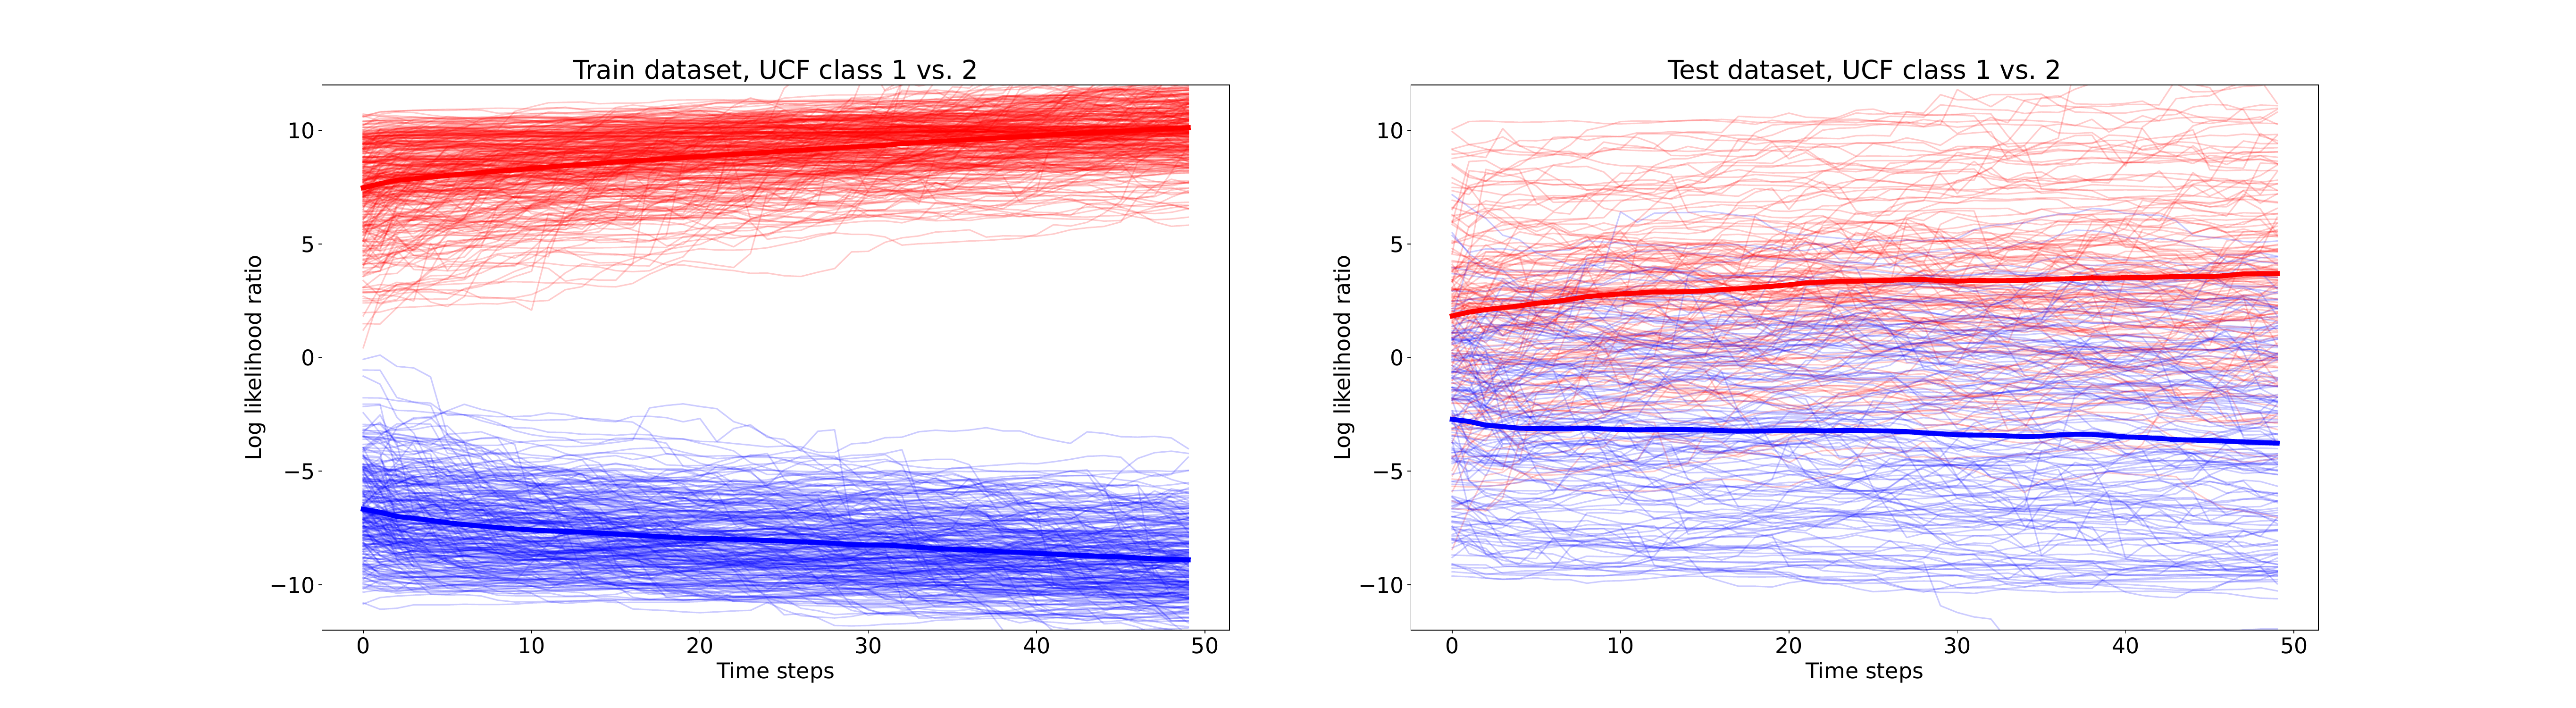}}
\caption{\textbf{Estimated LLRs on the train and test datasets of UCF101.} }
\label{fig:UCF_domain_gap}
\end{figure*}

\begin{figure*}[htbp]
\centerline{\includegraphics[width=14cm,keepaspectratio]{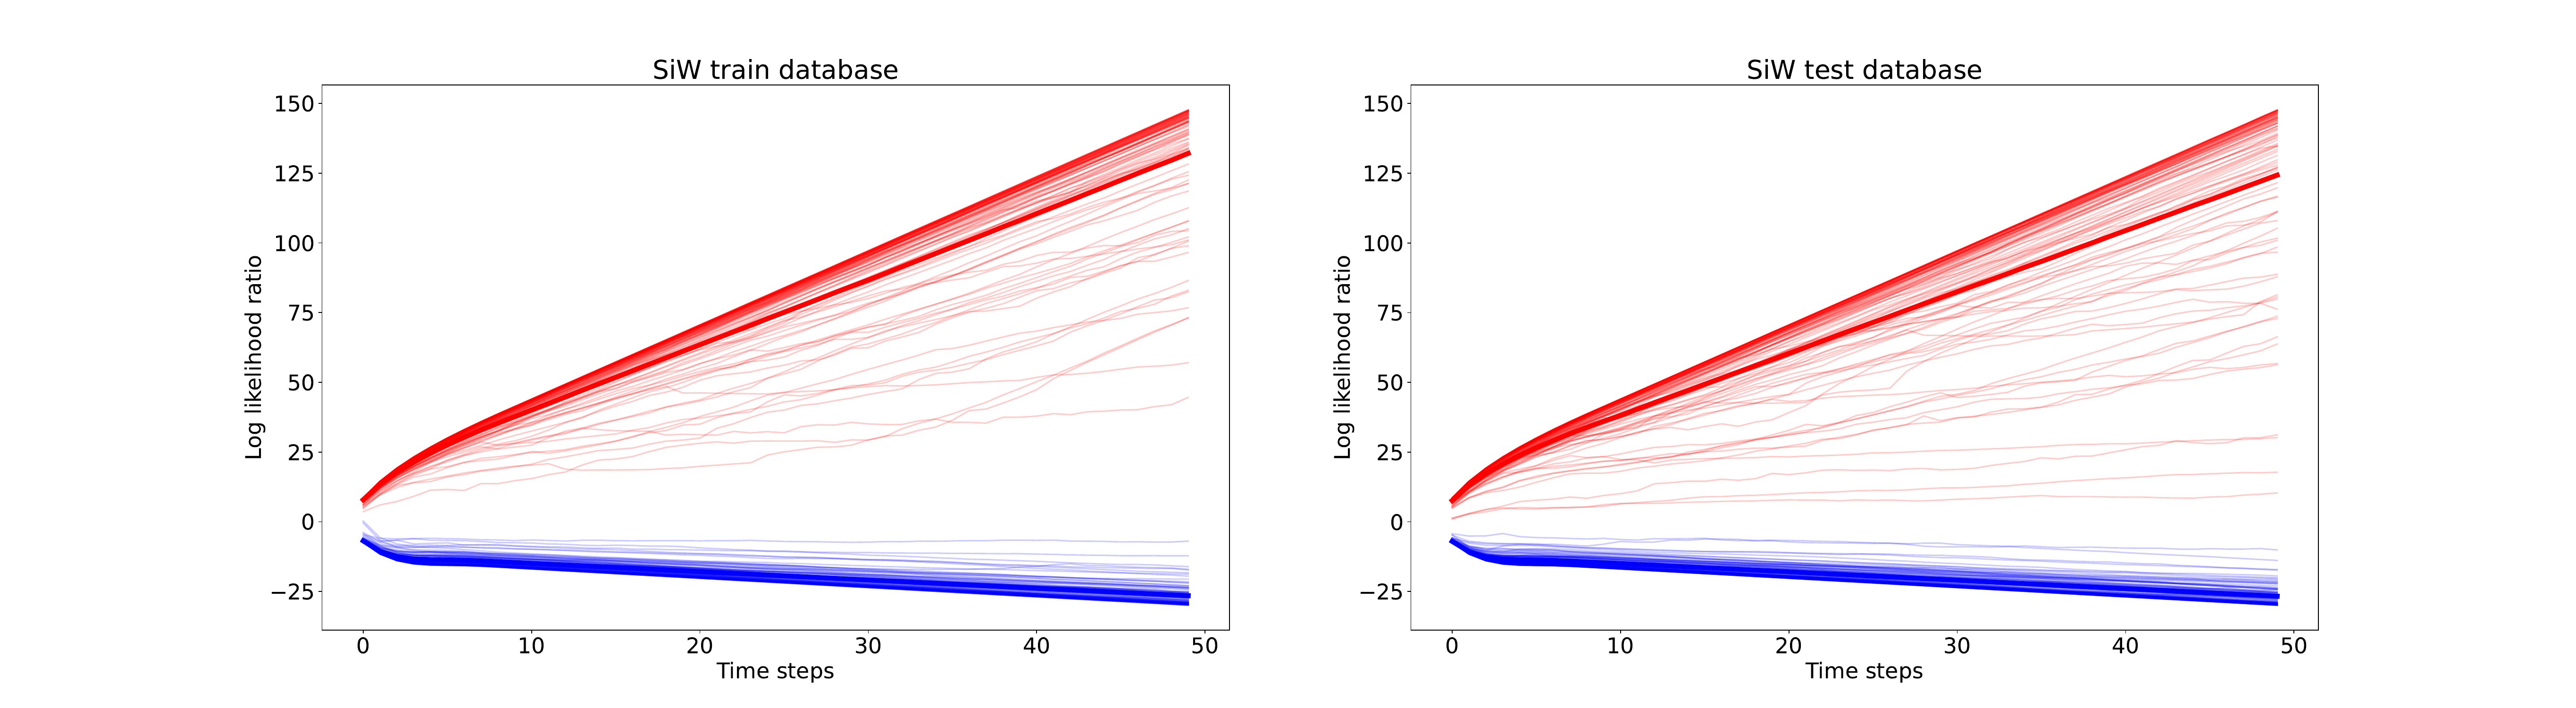}}
\caption{\textbf{Estimated LLRs on the train and test datasets of SiW.} }
\label{fig:SiW_domain_gap}
\end{figure*}

We recognize the importance of addressing domain gaps in machine learning research. However, it is important to note that handling domain gaps is beyond the current scope of our paper, which focuses on developing an optimal stopping rule for early classification within finite horizons. Addressing domain adaptation and transfer learning would require a different methodological approach and additional research efforts. Potential directions include incorporating domain adaptation techniques and robustifying FIRMBOUND against such discrepancies.

\clearpage
